# Supplementary material for: Agility and Target Distribution in the Dynamic Stochastic Traveling Salesman Problem
Source: arXiv:2302.00243 source file (2023-02-01)
Supplement: Supplementary file 1 [file 02_001_meta_assumption_redux.tex]

\documentclass[../main_file.tex]{subfiles}
%\graphicspath{{\subfix{../images/}}}
\begin{document}

In this appendix, we show how, if $\Pi$ is symmetric and control-affine, \Cref{meta:regularity} implies a number of our key assumptions. These are generally either well-known results from control theory or direct corollaries of well-known results; however, they can greatly simplify the process of checking whether a given control system satisfies the assumptions from \Cref{sec:assumptions}. We follow the definitions and notation from \emph{Control of Nonholonomic Systems: From Sub-Riemannian Geometry to Motion Planning} by Frederic Jean~\cite{jean-14}.

Since in this section we are working with symmetric control-affine systems, our basic control function will be
\begin{align}
    \dot{\bq} = \sum_{i=1}^m u_i h_i(\bq)
\end{align}
where $\bu = (u_1, \dots, u_m)$ is the control and the $h_i$ are $C^\infty$ vector fields over $\cspace$. We denote the space tangent to $\cspace$ at $\bq$ as $T_\bq \cspace$. 

We assume that $\bu$ is taken from some $\cU \subseteq \bbR^m$ which satisfies the following properties:
\begin{enumerate}
    \item $\cU$ is convex and full-dimensional;
    \item $\cU$ contains the origin $\bzero$ in its interior;
    \item $\cU$ is radially symmetric, i.e. $\bu \in \cU \iff -\bu \in \cU$.
\end{enumerate}

We then define $\vf(\cspace)$ as the set of smooth vector fields on $\cspace$; within this, $h_1, \dots, h_m$ generate a linear subspace which we denote
\begin{align}
    \Delta^{1} \defeq \spann\{h_1, \dots, h_m\} 
\end{align}
Letting $[a, b]$ denote the Lie bracket of $a, b$ (which denotes the direction of the motion produced by the commutator $a \circ b - b \circ a$), we then define $\Delta^s$ for all $s = 2, 3, \dots$ iteratively with
\begin{align}
    \Delta^s \defeq \Delta^{s-1} + [\Delta^1, \Delta^{s-1}]
\end{align}
and the Lie algebra generated by $h_1, \dots, h_m$ is
\begin{align}
    \lie(h_1,\dots,h_m) \defeq \bigcup_{s \geq 1} \Delta^s
\end{align}
i.e. all vector fields that can be produced by iterated Lie brackets and linear combinations from $h_1, \dots, h_m$. The Lie bracket $[a,b]$ denotes a direction of movement which can be produced by properly applying backwards and forwards motion (on small scales) of $a,b$; thus, a control-affine system which can move along $a,b$ can also move along $[a,b]$ though slower (for instance, if it can move $\varepsilon$ along $a,b$ per $\varepsilon$ time, then it can move $\varepsilon^2$ along $[a,b]$ per $\varepsilon$ time, note that it's not literally moving along $[a,b]$ continuously but doing a sequence of movements along $a$ and $b$ which eventually put it at a point on the flow of $[a,b]$). 

This then allows us to define \emph{Chow's condition}:
\begin{definition}
    Vector fields $h_1, \dots, h_m$ satisfy Chow's Condition if
    \begin{align}
        \lie(h_1,\dots,h_m) = T_\bq (\cspace) ~~~\text{for all } \bq \in \cspace
    \end{align}
\end{definition}
That is, Chow's Condition indicates that iterated Lie brackets can produce any direction at $\bq$ from $h_1,\dots,h_m$; this then yields the Chow-Rashevskii Theorem (\cite{jean-14}, Theorem 1.1) which states that if $\cspace$ is connected and satisfies Chow's Condition, the control-affine system can produce a point-to-point trajectory between any $\bq, \bq' \in \cspace$.

\end{document}
